# Supplementary material for: Industry Scale Semi-Supervised Learning for Natural Language Understanding
Source: arXiv:2103.15871 source file (2021-03-29)
Supplement: Supplementary file 1 [file appendix.tex]

\label{sec:appendix}
\section*{Appendix}
\section{Mathematical and Implementation Details for VAT and CVT}

% \subsubsection{Pseudo Label}
% Pseudo-label (PL) based self-training is a simple and straightforward method of SSL~\cite{yarowsky1995unsupervised,mcclosky2006effective}. Using a labeled dataset $\mathcal{D}_l$, we first train a model, $f_\theta$, to which we refer as a ``teacher'' model. We then generate a dataset of pseudo-labeled data from $\mathcal{D}_u$, by assuming that for each input instance $x_u$, the label $\hat{y}$, predicted by the teacher, is the correct label. The pseudo-labeled data is then incorporated to the training data, and a new model, to which we refer as a ``student'', is trained on the union of both datasets.

% \subsubsection{Knowledge Distillation}
% In Knowledge Distillation (KD), for a given input $x$, a teacher model produces a probability distribution over all possible labels, $l \in \mathcal{L}$, where $\mathcal{L}$ refers to the label space. The predicted probability distribution is often referred to as ``soft label''. The student model is then trained alternating between two objectives: minimizing the loss on the labeled data, defined respectively for different tasks, and minimizing the cross-entropy loss between the student and teacher predicted ``soft label'' on the unlabeled data. In other words, the student model learns from the predicted distribution over labels instead of a predicted label. 

% The soft labels on intents are generated by the IC task softmax layer, while the soft labels on label sequences are generated per token, by running softmax on the logits for each token before the CRF layer. 

\subsection{Virtual Adversarial Training}
% Virtual adversarial training (VAT) is an efficient semi-supervised approach based on adversarial learning~\cite{vat}. It has been shown to be highly effective in both image~\cite{vat} and text classification~\cite{vat_classification} tasks. Given an unlabeled instance, VAT generates a small perturbation that would lead to the largest shift on the label distribution predicted by the model. After getting the adversarial perturbation, the objective is to minimize the KL divergence between the label distribution on the original instance and the instance with perturbation. 

Let $x$ denote an input to the model, $y$ the corresponding label, and $\theta$ the model parameters; the loss, $L$, for VAT can be written as:

\begin{equation}\label{eqn:vat_kl}
    L_{vat} = D_{KL} \big(\hspace{0.1cm} P(\hat{y};x,\hat{\theta})\hspace{0.1cm} ||\hspace{0.1cm} P(\hat{y}; x+d,\hat{\theta})  \big)\nonumber
\end{equation}

\noindent where $d$ stands for the adversarial perturbation, and $P$ stands for the label distribution for a given input and parameters. The notation $\hat{y}$ and $\hat{\theta}$ is used to emphasize that the computation of KL divergence takes current estimation of label distribution and parameters.

And the worst-case perturbation can be computed by:
\begin{equation}\label{eqn:perturb_word_vat}
     d = \operatornamewithlimits{argmax}\limits_{\epsilon,||\epsilon||_2 \leq \delta} D_{KL}(P(\hat{y};x,\hat{\theta})  ||
     P(\hat{y};x+\epsilon,\hat{\theta})) \nonumber
 \end{equation}
 where $\delta$ is the bounded norm for adversarial perturbations.

 \noindent With VAT loss, the training loss is:
 \begin{equation}\label{eqn:vat_total_loss}
     L = L_{supervised} + \alpha * L_{vat} \nonumber
 \end{equation}

 \noindent $\alpha$ is the weight used to balance supervised loss and VAT loss. In our experiments, $\delta$ is set to 0.4 and $\alpha$ is set to 0.6.

 \subsection{Cross-View Training}
% Cross-view training (CVT) is another SSL approach proved to be efficient on text classification, sequence labeling and machine translation~\cite{cvt}. Using an bi-directional LSTM, CVT uses the prediction from the current state as an auxiliary prediction, takes the output from neighboring LSTM neurons in each direction and forces them to predict the same label as the current neuron. 
% % \begin{equation}\label{eqn:cvt_main}
% %     \hat{y} = Softmax(NN([f_i; b_i]))
% % \end{equation}

Let $f_i$ be the forward output from step $i$ and $b_i$ as the backward output from step $i$. The auxiliary prediction can be written as: $\hat{y} = Softmax(NN([f_i; b_i]))$. Then $\hat{y}$ would be used as ground truth for 4 adjacent states, and calculate cross entropy (CE) loss:

 \begin{eqnarray}\label{eqn:cvt_loss}
 L_{forward} = CE(\hat{y}, \hspace{0.1cm}Softmax(NN^{forward}(f_i))) \nonumber\\
 L_{backward} = CE(\hat{y}, \hspace{0.1cm}Softmax(NN^{backward}(b_i))) \nonumber\\
 L_{past} = CE(\hat{y}, \hspace{0.1cm}Softmax(NN^{past}(f_{i-1}))) \nonumber\\
 L_{future} = CE(\hat{y}, \hspace{0.1cm}Softmax(NN^{future}(b_{i+1})))\nonumber
 \end{eqnarray}
 The final CVT loss is the mean of them:
 \begin{equation}\label{eqn:cvt_total}
     L_{cvt} = \frac{1}{4} * (L_{forward} + L_{backward} + L_{past} + L_{future} )\nonumber
 \end{equation}
 And the training loss is:
 \begin{equation}\label{eqn:cvt_total_loss}
     L = L_{supervised} + \beta * L_{cvt}\nonumber
 \end{equation}

 \noindent $\beta$ is the weight used to balance supervised loss and CVT loss. In our experiments, $\beta$ is set to 0.8.

\section{SSL Training Data Set Size}
To investigate how the size of the SSL training data set could impact the performance, we select KD based SSL, and carry out a series of experiments on Music domain, with SSL training data set size ranging from 10k to 1m, while keeping the labeled data set at 50k. All training data are randomly selected from the SSL data pool. %The results are shown in Table \ref{SSL Data Set Size}. 

It is observed that performance improvement from SSL generally increases with the size of SSL training data set; more SSL training data not only facilitates the transfer of knowledge between teacher and student models, it also exposes the student model to more speech pattern varieties. However, after a certain level, increasing SSL training data size degrades performance improvement. Because SSL data is inherently noisy and contains errors made by the teacher model, it is important to maintain a balance between labeled data and SSL training data. In our setting, we observe 500k as an optimal size for SSL training data set, with respect to 50k labeled training data. 
% In data selection experiments, we explore, out of the 500k data pool, how can we further select the data points which are more beneficial to model training, thus improving the training efficiency as well as optimizing the model performance. 

%\textcolor{red}{Diversity based on unigrams might not tell the whole story. In domains that are entity rich, you could have higher diversity in unigrams/n-grams, but the utterances are similar. We should try to say something a bit more insightful here.}

\begin{table*}[ht]
\small{
\caption{\label{table:ngram_diversity} Unique unigram and 1-4 grams ratio present in $\mathcal{D}_l \cup \mathcal{D}_u$ and $\mathcal{D}_l$}
\begin{center}
\begin{tabular}{c|c|c|c|c|c|c}
\hline 
\multirow{2}{*}{Domains} & \multicolumn{2}{c|}{Random} & \multicolumn{2}{c|}{Committee} & \multicolumn{2}{c}{Submod} \\ 
\cline{2-7} 
& \multicolumn{1}{c|}{Unigram} & \multicolumn{1}{c|}{1-4 gram} & \multicolumn{1}{c|}{Unigram} & \multicolumn{1}{c|}{1-4 gram} & \multicolumn{1}{c|}{Unigram} & \multicolumn{1}{c}{1-4 gram} \\ \hline 
Communication & 3.21 & 9.29  &	\textbf{3.29} & \textbf{10.21} & 1.41 & 6.17 \\ 
Todos         & \textbf{2.88} &	\textbf{6.04} &  1.4  & 3.51  & 1.51 & 3.19 \\
Music         & 3.19 &  6.42 &	3.24 & 6.39  & \textbf{3.43}	& \textbf{7.18} \\ 
Notifications & 3.04 &  \textbf{6.01} &	\textbf{3.08} & 5.9   & 1.77	& 3.97 \\ 
\hline 
\end{tabular}
\end{center}}
\end{table*}

\section{Diversity Analysis of SSL Data}

In order to understand how different data selection methods behave, we conduct an additional analysis on diversity of the selected data set, based on n-gram overlap between labeled and selected unlabeled data.

% While random selection uniformly selects the data, both submodular selection and committee based selection approach selects data non-uniformly. 
In supervised machine learning, a diverse training set often correlates with good generalizability. To understand the correlation between the diversity of SSL training data set and model performance, we measure the diversity of the selected data by computing the unique n-gram ratio present in $\mathcal{D}_l \cup \mathcal{D}_u$ and $\mathcal{D}_l$ data. This provides a sense of how different the selected data is from the data used for training. The higher the ratio, the more diverse the n-grams of unlabeled data are compared to the labeled data. Table \ref{table:ngram_diversity} shows the unigram and 1-4 gram ratios for the different selection algorithms. Unigram ratio of $2$ means that a selection algorithm has expanded the vocabulary size by two. Similarly 1-4 gram ratio represents the ratio by which n-gram vocabulary has expanded. We observe that a diverse ssl pool does not necessarily lead to better performance. For example, in Todos domain, while randomly selected data is more diverse, committee based selection consistently outperforms random on both IC and NER task. This result highlights that simply optimizing for token diversity is not enough for improving SSL performance.

\section{Full Results on SNIPS Dataset}

The full test results with different data selection approaches are shown in table \ref{Full Snips SSL Comparison}. Both submodular optimization based selection and committee based selection do not bring additional improvements over random selection. Note than unlike commercial dataset, here SSL data is very different from the SNIPS data. Since, submodular optimization based selection tries to select diverse n-grams present in labeled as well unlabeled data, submodular selection is prone to pick utterances which are not related to the task. Consequently, the selected data is not guaranteed to be better than random selection. On other hand, committee based selection relies on having a representative dev set to find robust cutoff threshold for the entropy. Since, SNIPS dev set is very small (700 utterances) committee based selection's entropy cutoff is not very reliable. Thus the quality of selected data is not better than the random selection.

\begin{table}[h]
\caption{\label{Full Snips SSL Comparison} Model performance by different SSL methods and data selection methods, for SNIPS data set. The metric for IC task is intent classification error rate. The metric for NER task is entity recognition F1 error rate.  }
\begin{center}
\small{
\begin{tabular}{c|c|c|c}
\hline 
SSL & Selection & \multicolumn{2}{c}{SNIPS} \\ 
\cline{3-4} 
 Algorithm &  Approach & \multicolumn{1}{c|}{IC} & \multicolumn{1}{c}{NER}  \\ \hline 
Baseline &  & 0.9744 & 0.9367  \\ 
PL &  & 0.9743 & 0.9326  \\
KD & Random & 0.9743 & 0.9424   \\
VAT &  & 0.9814 & \textbf{0.9604}  \\
CVT &  & \textbf{0.9871} & 0.9565 \\ \hline 

Baseline &  & 0.9744 & 0.9367   \\ 
PL &  & 0.9743 & 0.9342  \\
KD & Submodular & \textbf{0.9786} & 0.9403  \\
VAT &  & 0.9728 & \textbf{0.9579}  \\
CVT &  & 0.9785 & 0.9524 \\ \hline 

Baseline &  & 0.9744 & 0.9367   \\ 
PL &  & 0.9700 & 0.9272  \\
KD & Committee & 0.9729 & 0.9353  \\
VAT &  & 0.9772 & 0.9501  \\
CVT &  & \textbf{0.9780} & \textbf{0.9518} \\ \hline 

\end{tabular}}
\end{center}
\end{table}

\section{Comparison of Data Selection Strategies}
In terms of data selection strategies for SSL, both submodular-based selection and committee-based selection bring an added benefit over randomly selected data. There is a clear reason that would explain this difference. In live traffic, the distribution of data is far from uniform. Certain intents and entities are requested a lot more often than others. Furthermore, many utterances might be distinctive, but they could simply be background noise or requesting functionalities not yet supported.
Therefore, data sampled at random from live traffic is likely to contain many utterances with similar patterns, and utterances that are not supported by the system, thus should not be used for SSL. Submodular-based selection addresses the first of these problems by filtering out utterances which add little value to the model, while committee-based selection addresses the second by filtering out utterances for which the committee has low confidence, indicating they could be out of domain data.

Submodular techniques are cheap to run, so when debating whether to randomly sample data for SSL techniques or use submodular-based data selection, our recommendation is to use the submodular approach. The decision between submodular and committee-based selection is more nuanced. The submodular approach will try to increase diversity of the data selected, and try to find representative examples of the unlabeled pool of data. This might result in selecting samples that differ significantly from the training data. If the model is able to produce reasonable predictions, selecting diverse data points would be beneficial. If the model is not able to do so, incorporation of data points with noisy annotation could hinder improvement. In other words, this is a more optimistic data selection approach. On the other hand, committee-based selection takes a more conservative approach, where the data selected is likely to be annotated correctly by the teacher models.

\begin{table*}[h]
\caption{ Performance of models trained using different SSL techniques, for SNIPS data set. The metric for IC task is intent classification error rate. The metric for NER task is entity recognition F1 error rate. Mean and Std of model trained with 3 randomly selected SSL data sets are displayed. }
\begin{center}
\small{
\begin{tabular}{c|c|c|c|c|c}
\hline 
Task & Baseline & PL & KD & VAT & CVT \\ \hline 
IC & 0.9744 & 0.9762 $\pm$ 0.0022 & 0.9738 $\pm$ 0.0022 & 0.9814 $\pm$ 0.0028 & \textbf{0.9872 $\pm$ 0.0012} \\
NER & 0.9367 & 0.9305 $\pm$ 0.0023 & 0.9394 $\pm$ 0.0026 & \textbf{0.9608 $\pm$ 0.0009} & 0.9566 $\pm$ 0.0017 \\ \hline 

\end{tabular}}
\end{center}
\end{table*}

\emph{Which data selection method should one use?} Based on our experiments, if training cost is not a concern and poor SSL annotated data could be too detrimental, committee-based selection would provide a good balance between improvements on SSL methods without being too aggressive on its data selection. On the other hand, if the cost of training a committee is too expensive, one might consider using submodular-based data selection.

In order to understand how different data selection methods behave, we examine the effect they have on under-represented categories of data. Within each domain, there are several intents representing the different goals the user might try to achieve. A small number of the available intents are used much more frequently than the rest, representing the majority of the data available for training and testing in that domain. %For example, in the Music domain, PlayMusicIntent is used much more frequently than MusicControlIntent which is used for switch/shuffle/replay operations. 
%\textcolor{red}{I comenent out the example between PlayMusicIntent and MusicControlIntent to avoid exposing intent name and distribution}
Given this imbalance in intent distribution, SSL trainings are more likely to be carried out with poor quality SSL data for intents that are not encountered very frequently. As such, the performance improvements seen overall might only be the result of improving over-represented intents, or worse, might come at the cost of performance degradation for under-represented intents. 

Filtering data based on confidence, as done in committee-based selection, should address this problem by preventing poorly annotated data to be included as SSL training data. For this experiment, we identify three under represented intents for Music, Communication, and Notifications domains, respectively. We have between $100$ and $1,000$ labeled utterances for each of the intents. In comparison, the most frequently used intents have more than $5,000$ and up to $10,000$ samples. The effect of committee-based data selection becomes evident from observing table \ref{table:mid-intents}, where we compare its effects to random and submodular data selection while using KD as our SSL technique. The table compares the f1 score of the selected under-represented intents, relative to a baseline trained with only labeled data. Notice that unlike in previous tables showing error reduction, in this table we report f1 score improvement, hence higher numbers indicate better performance.

\begin{table}[t]
\caption{\label{table:mid-intents} Performance comparison for under-represented intents using different data filtering methods. Changes in intent recognition F1 score, relative to baseline, are reported. }
\begin{center}
% \scriptsize{
% {\fontsize{7.5}{7.5}\selectfont 
\small
\begin{tabular}{c|c|c|c}
\hline 
Intents & Random & Submodular & Committee   \\ \hline 
%CreatePlaylistIntent 
Music\_A &  -0.49\% & \textbf{1.95\%} & 0.35\% \\ 
% AddToPlaylistIntent 
Music\_B & 0.78\% & \textbf{0.87\%} & 0.60\% \\ 
% MusicControlIntent 
Music\_C & 2.42\% & 2.95\% & \textbf{3.72\%} \\
% EndCallIntent
Communication\_A & -0.64\% & -0.04\% & \textbf{2.73\%} \\ 
% GetMessageIntent
Communication\_B & 0.92\% & 1.25\% & \textbf{1.53\%} \\ 
% BrowseContactList
Communication\_C & 2.37\% & 1.32\% & \textbf{3.04\%} \\
% ExtendNotificationIntent
Notifications\_A & -0.74\% & -0.56\% & \textbf{2.59\%} \\
% EditNotificationIntent
Notifications\_B & 1.55\% & 0.79\% & \textbf{2.61\%} \\
% EnableNotificationInten
Notifications\_C & 1.01\% & \textbf{2.13\%} & 0.70\% \\

\hline 
\end{tabular}
\end{center}
\end{table}
Table \ref{table:mid-intents} shows that, while committee-based selection does not necessarily lead to the best improvements across all intents, comparing to submodular or random selection, it more consistently brings improvement for under-represented intent. Even though we observe larger improvements for submodular than for committee data selection for some intents, we also observe regression caused by submodular data selection for some other intents. In contrast, committee-based selection lead to stable or improved performance in all the under represented intent examples.
